# Supplementary material for: RethNet: Object-by-Object Learning for Detecting Facial Skin Problems
Source: arXiv:2101.02127 source file (2021-01-11)
Supplement: Supplementary file 1 [file cover_supp.pdf]

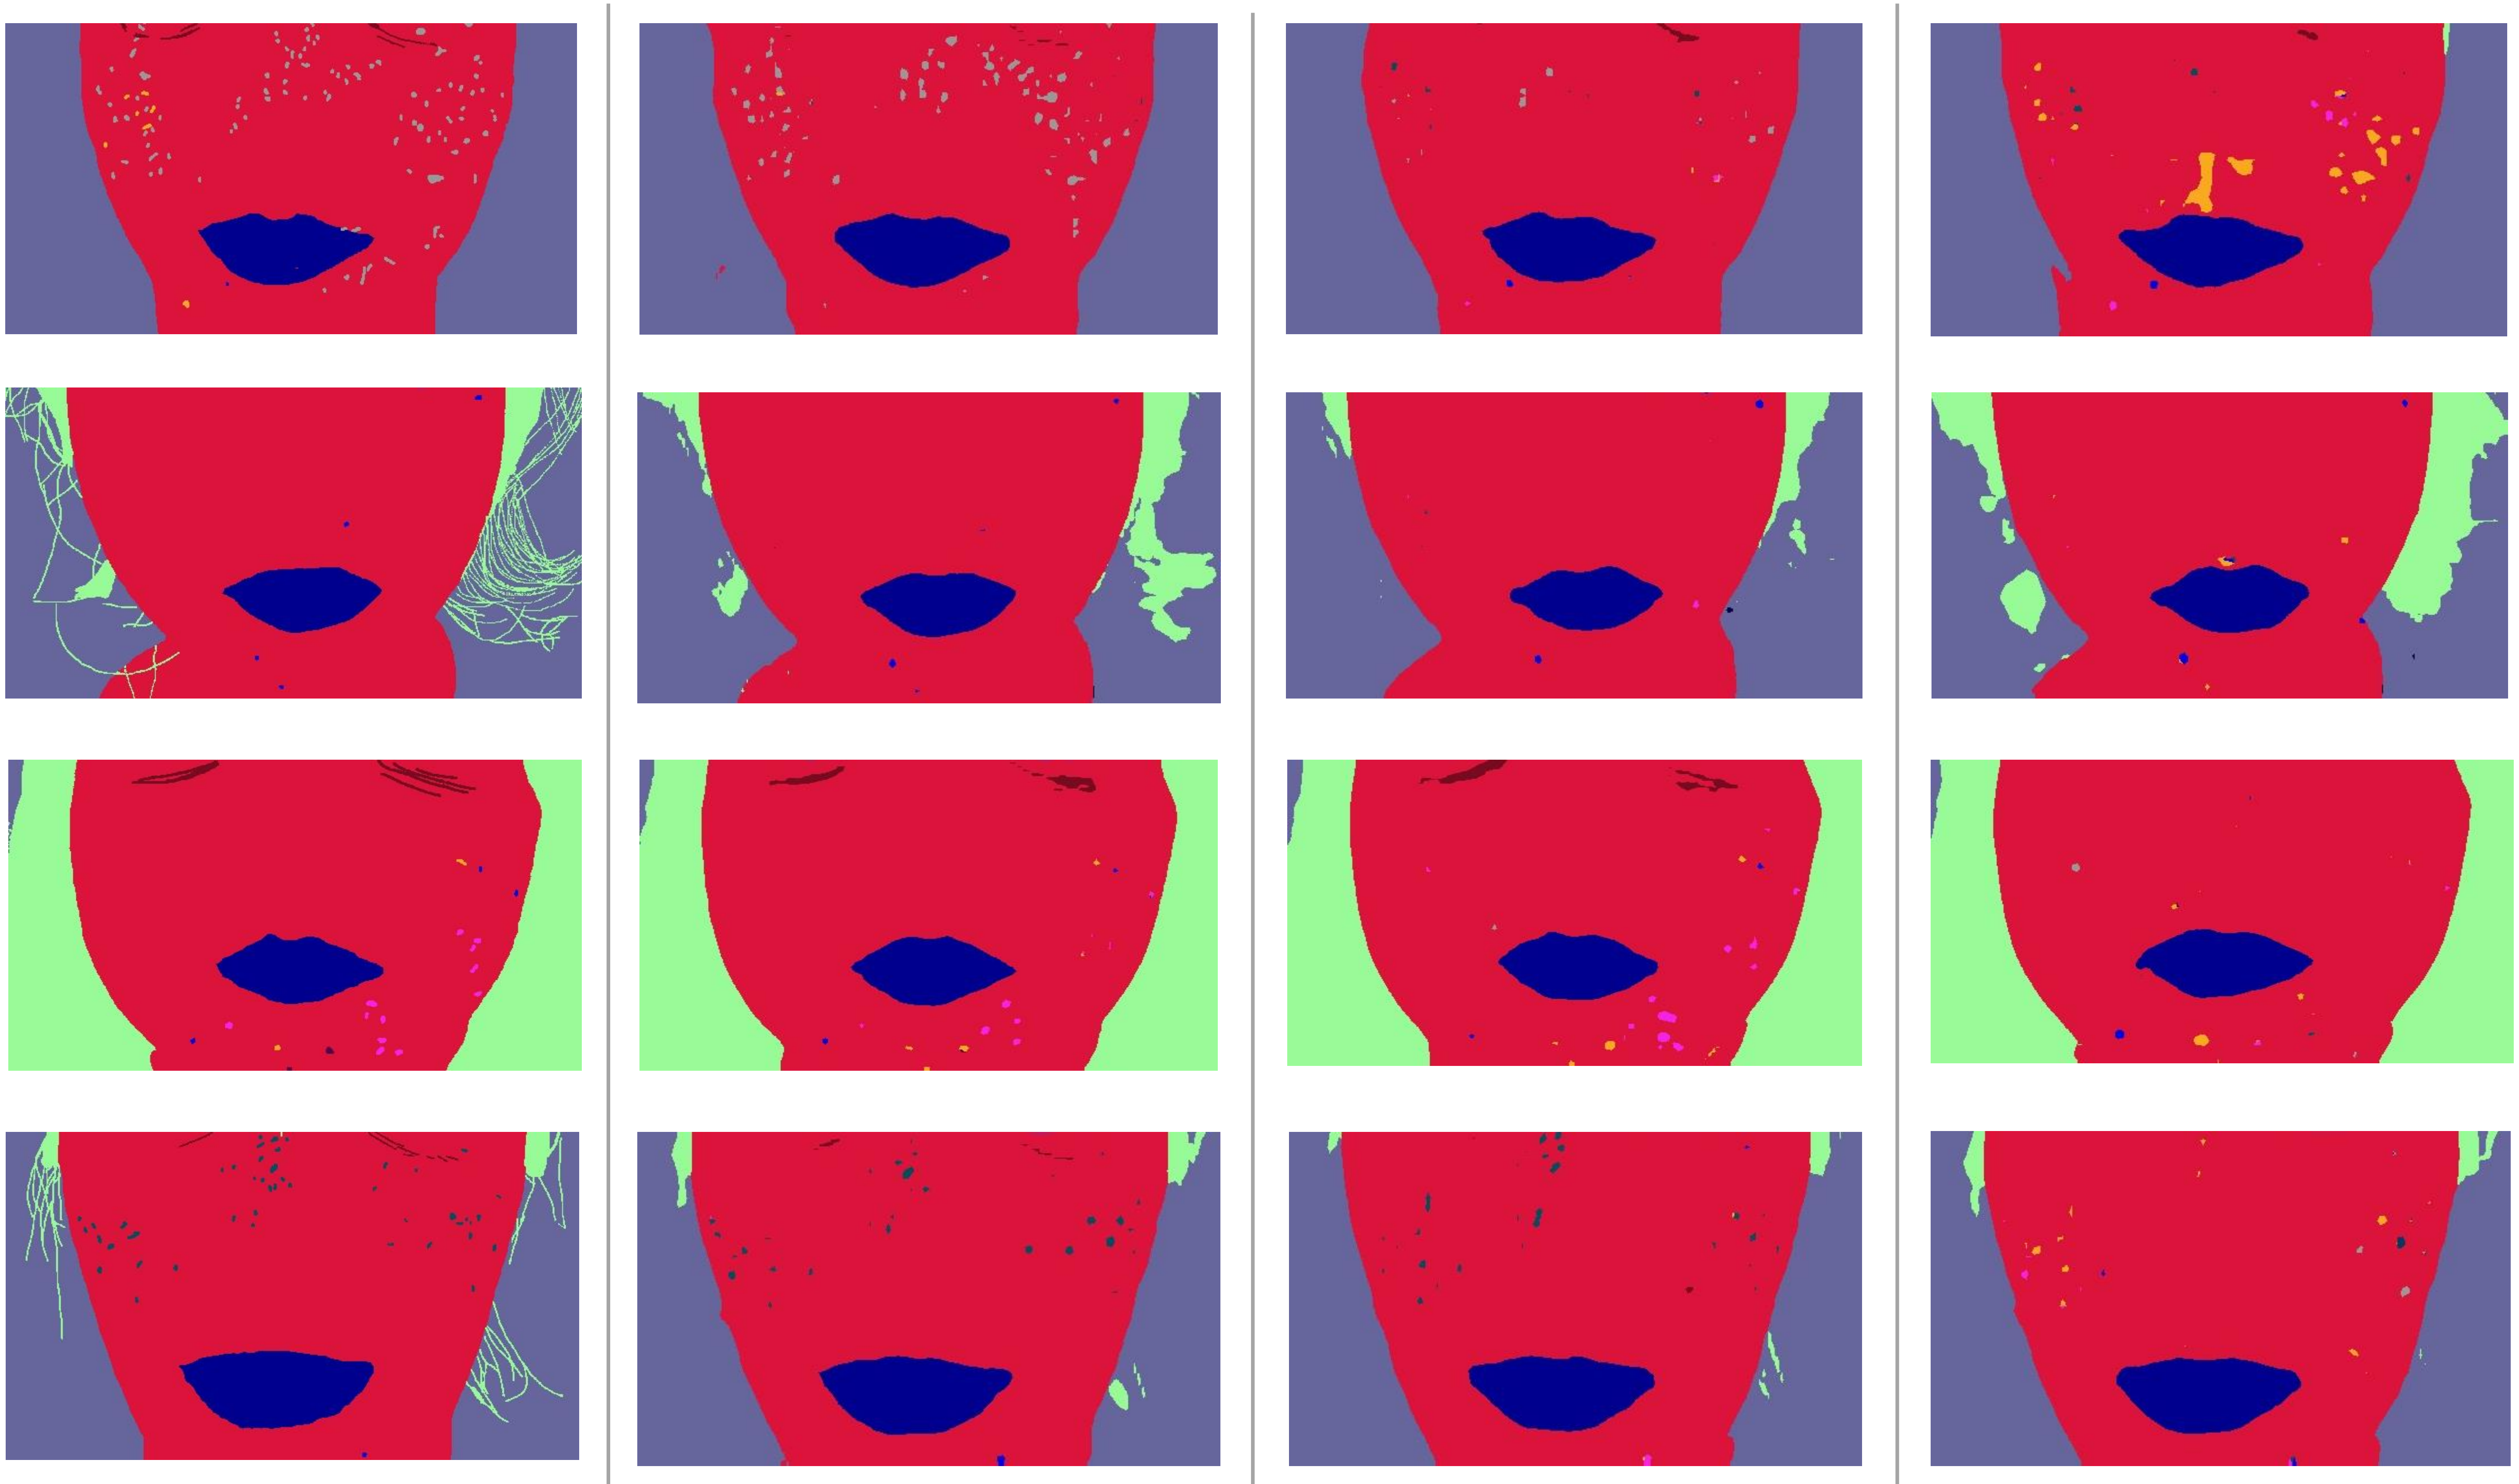

Ground Truth | RethNet + Rehtinker+e | RethNet + Rehtinker+d | Deeplab v3Plus + Xception

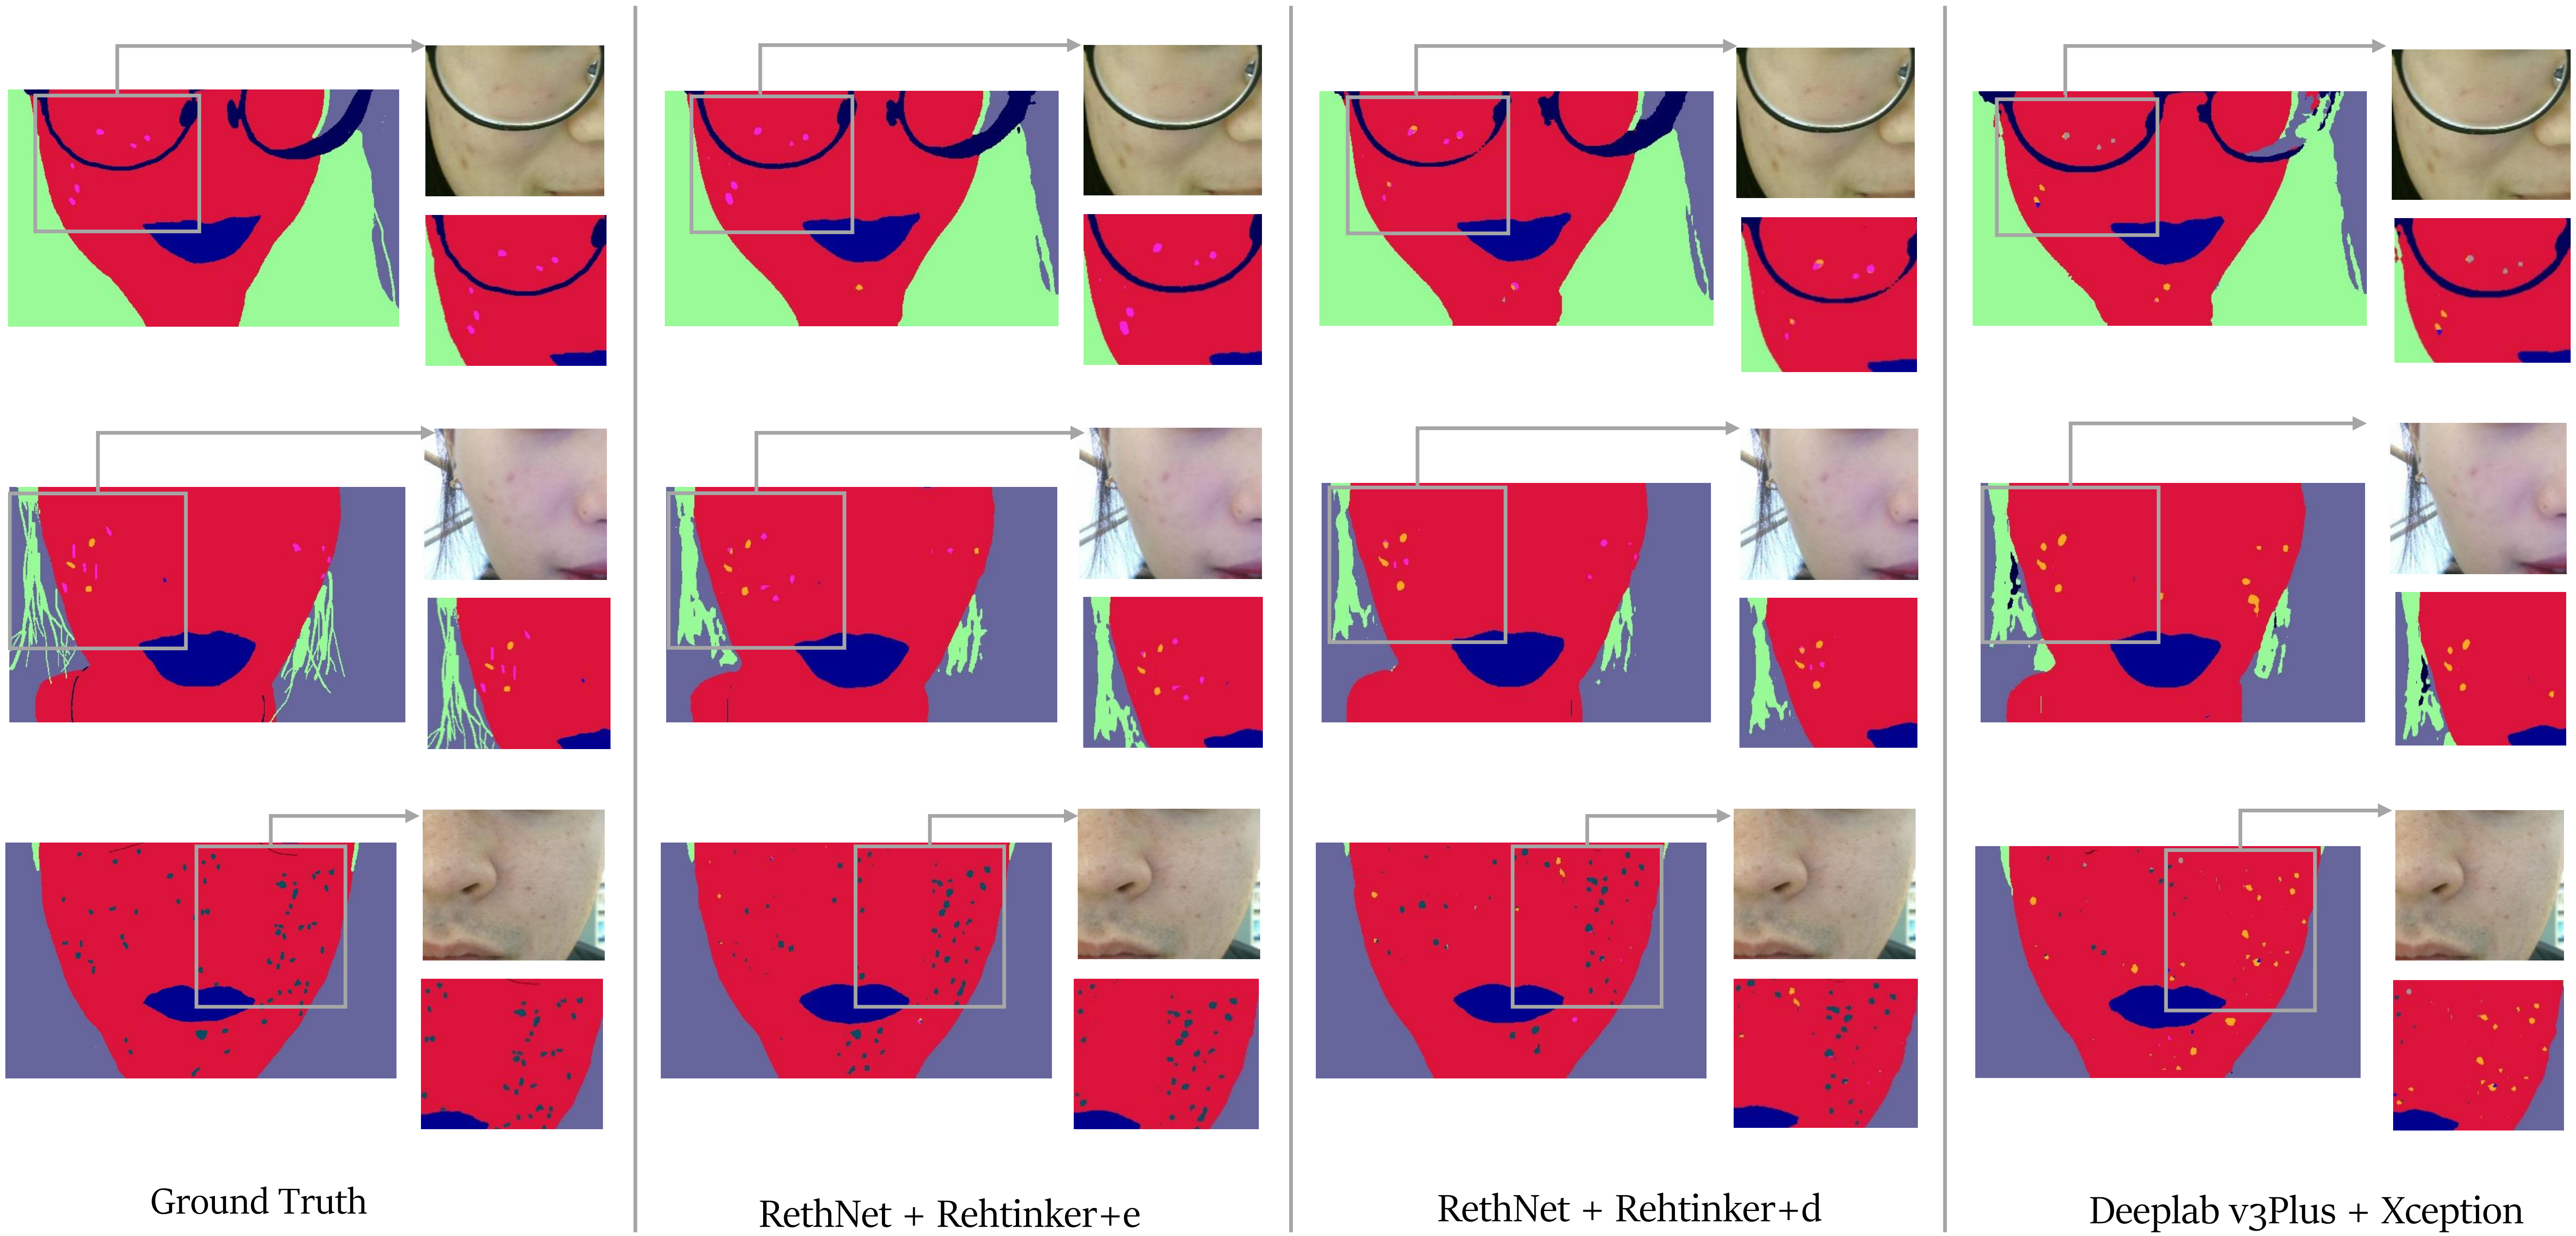
Ground Truth
RethNet + Rehtinker+e
RethNet + Rehtinker+d
Deeplab v3Plus + Xception

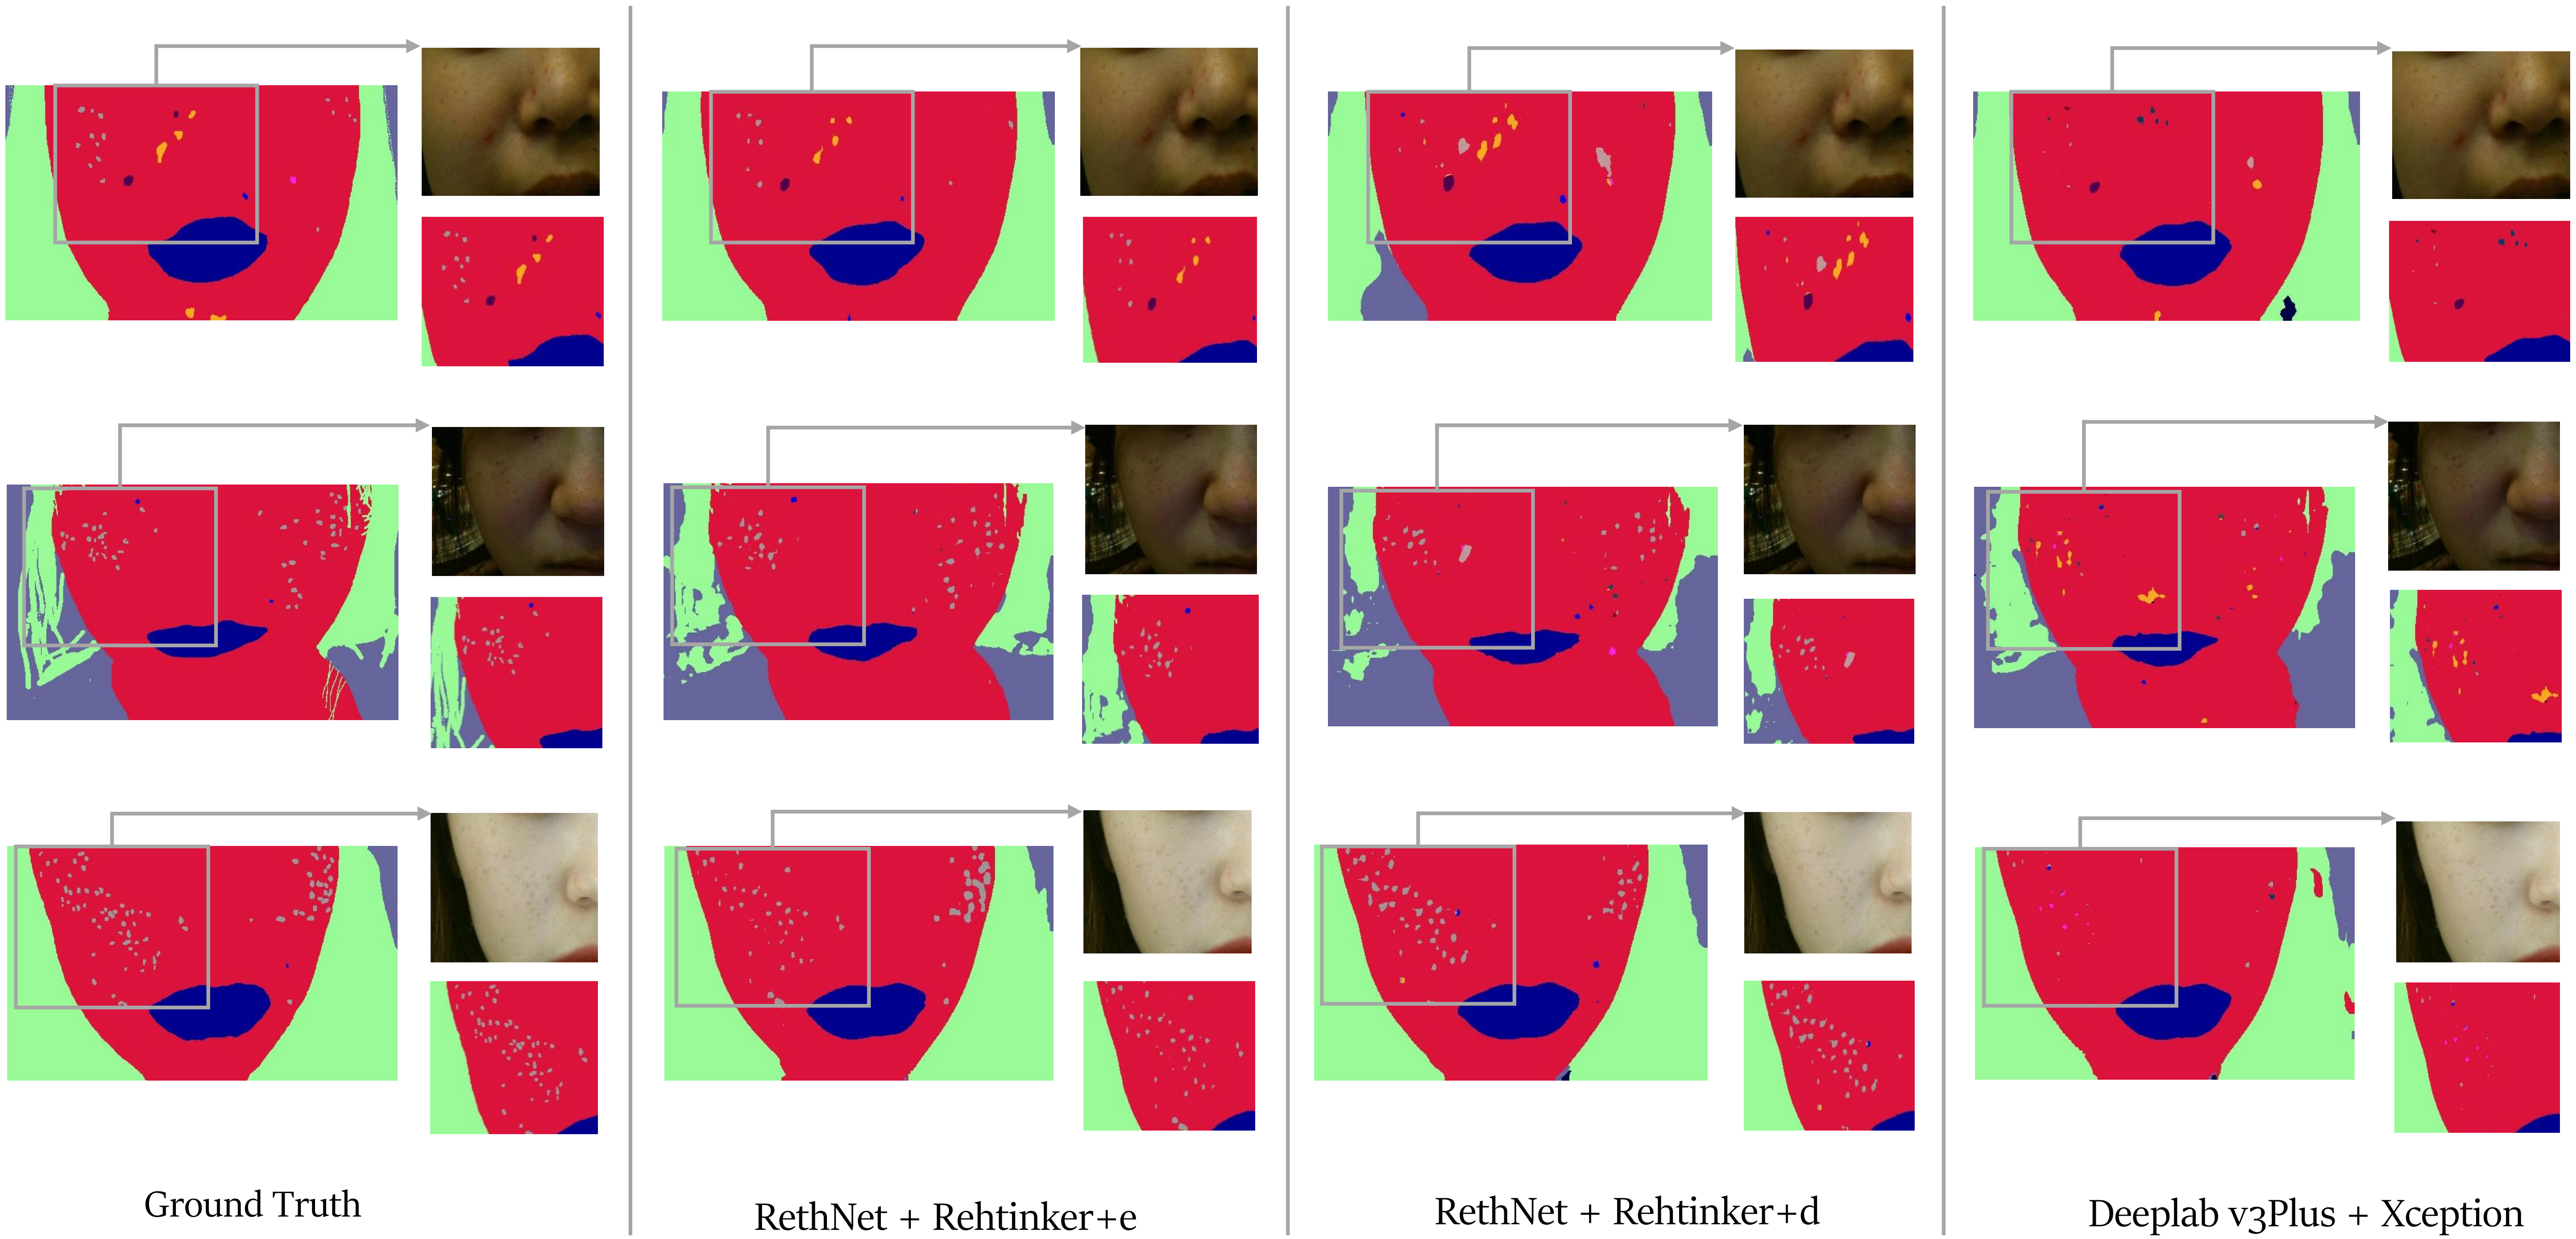

Ground Truth
RethNet + Rehtinker+e
RethNet + Rehtinker+d
Deeplab v3Plus + Xception

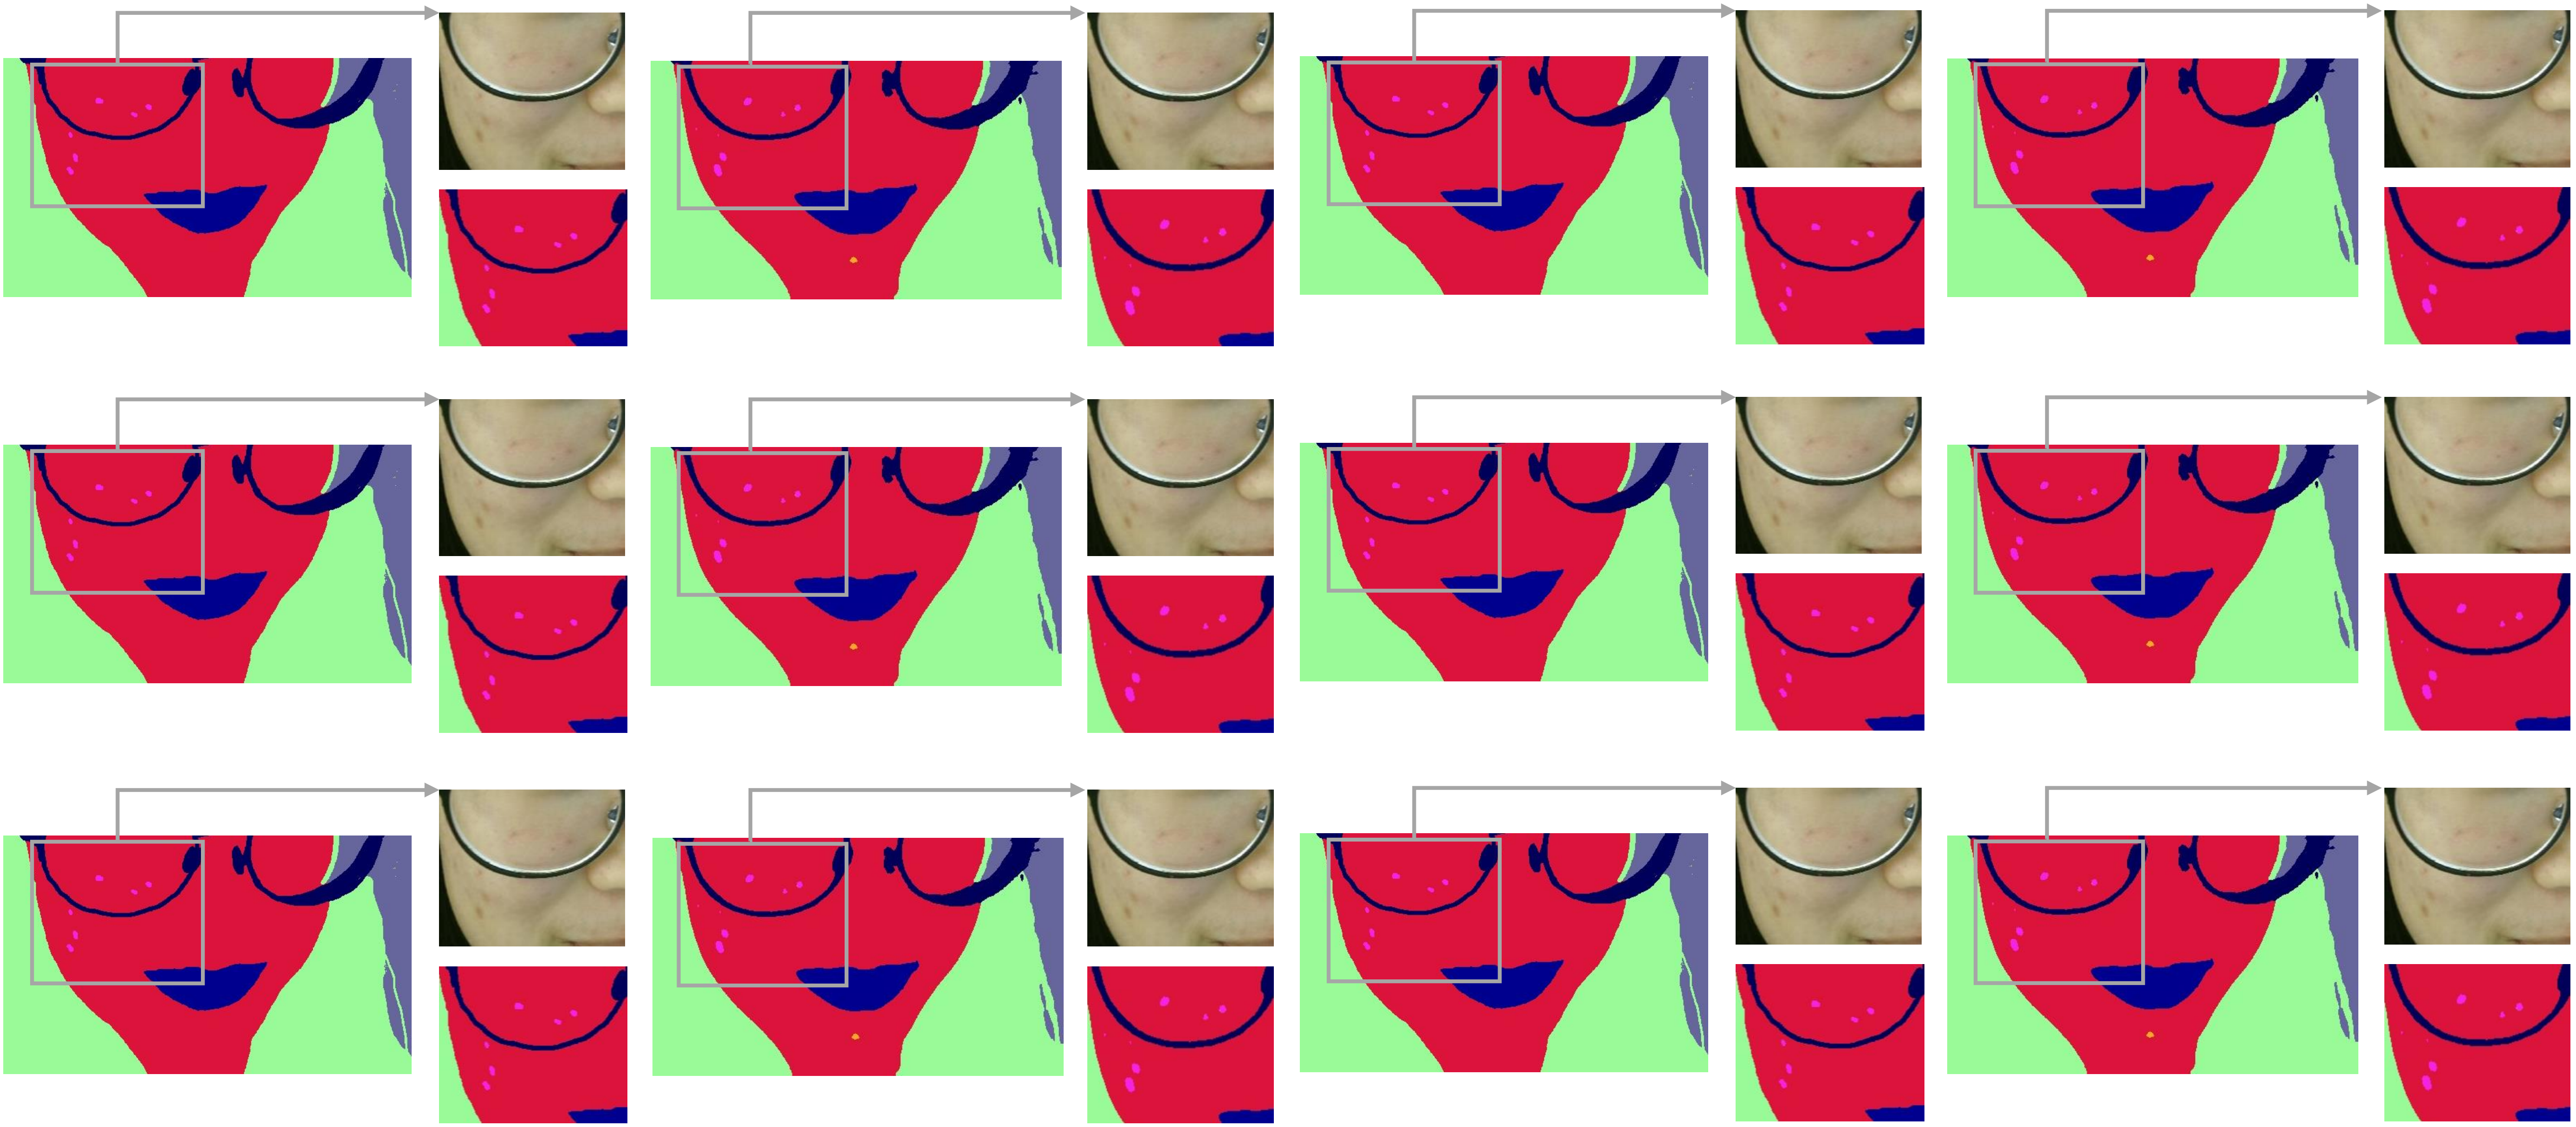

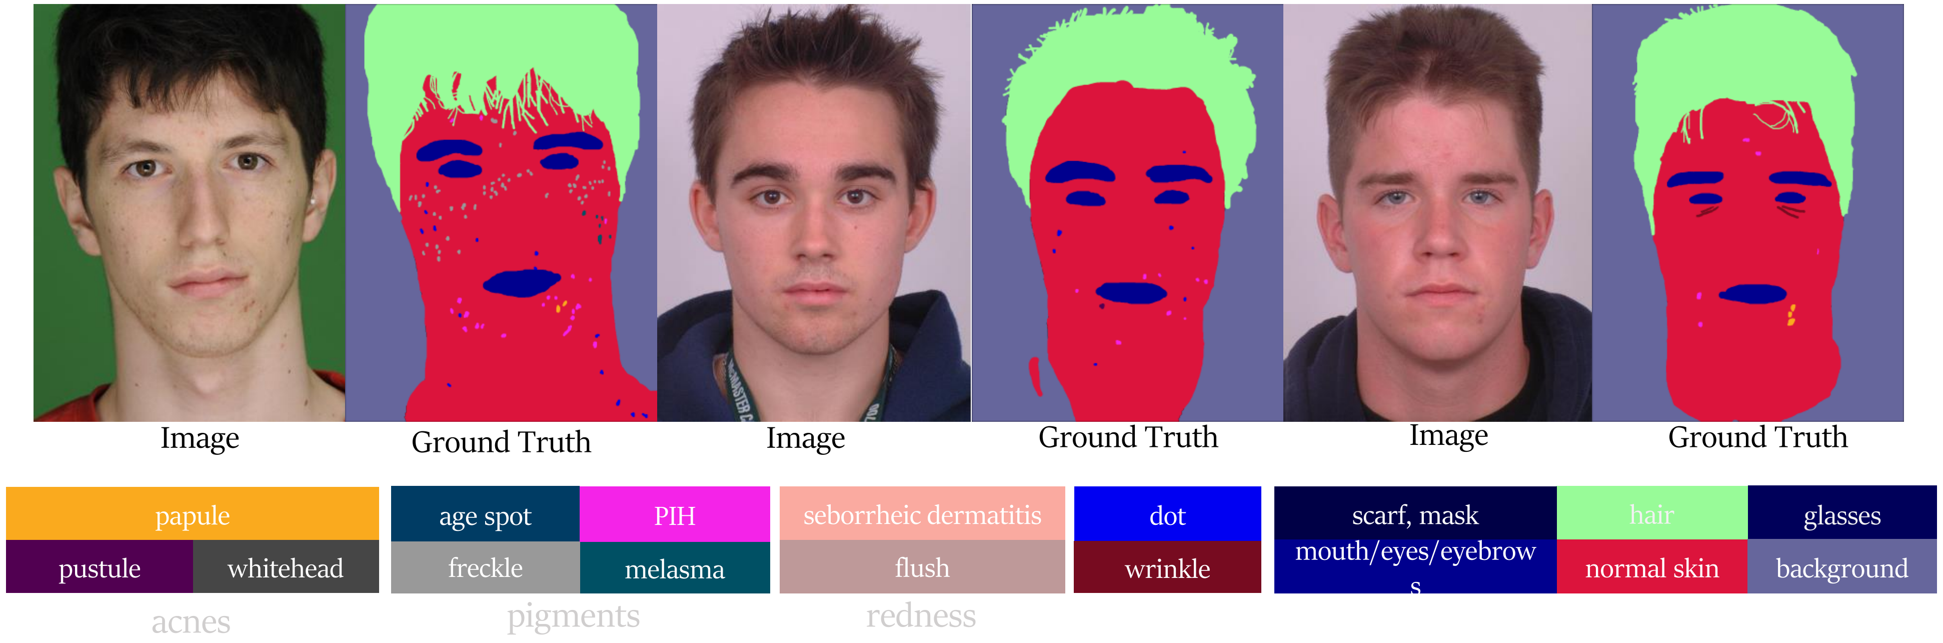

Image
Ground Truth
Image
Ground Truth
Image
Ground Truth
papule
pustule
whitehead
acnes
age spot
PIH
freckle
melasma
pigments
seborrheic dermatitis
flush
redness
dot
wrinkle
scarf, mask
mouth/eyes/eyebrow s
hair
glasses
normal skin
background

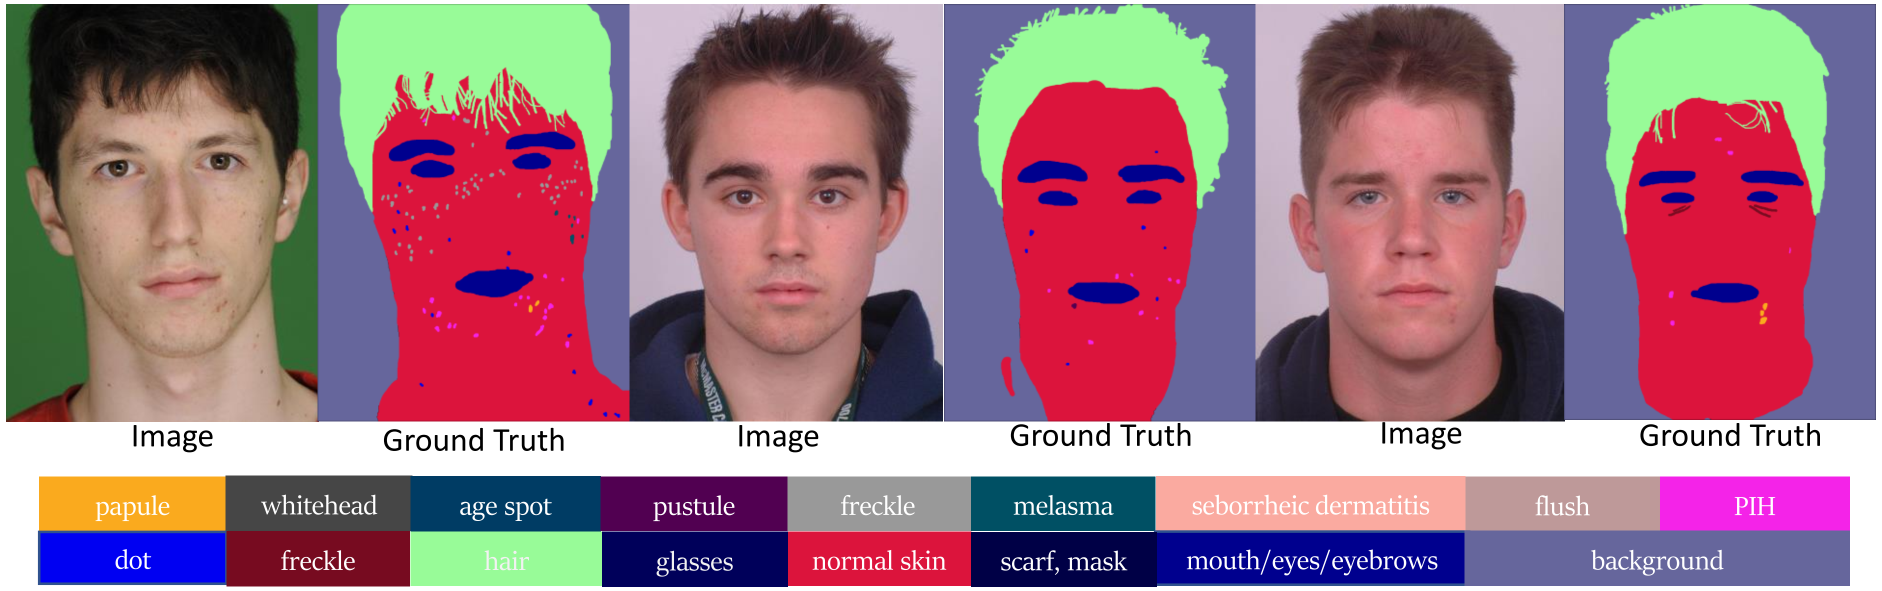
Image
Ground Truth
Image
Ground Truth
Image
Ground Truth
papule
whitehead
age spot
pustule
freckle
melasma
seborrheic dermatitis
flush
PIH
dot
freckle
hair
glasses
normal skin
scarf, mask
mouth/eyes/eyebrows
background
