# Supplementary material for: RethNet: Object-by-Object Learning for Detecting Facial Skin Problems
Source: arXiv:2101.02127 source file (2021-01-11)
Supplement: Supplementary file 4 [file supp_mat3.pdf]

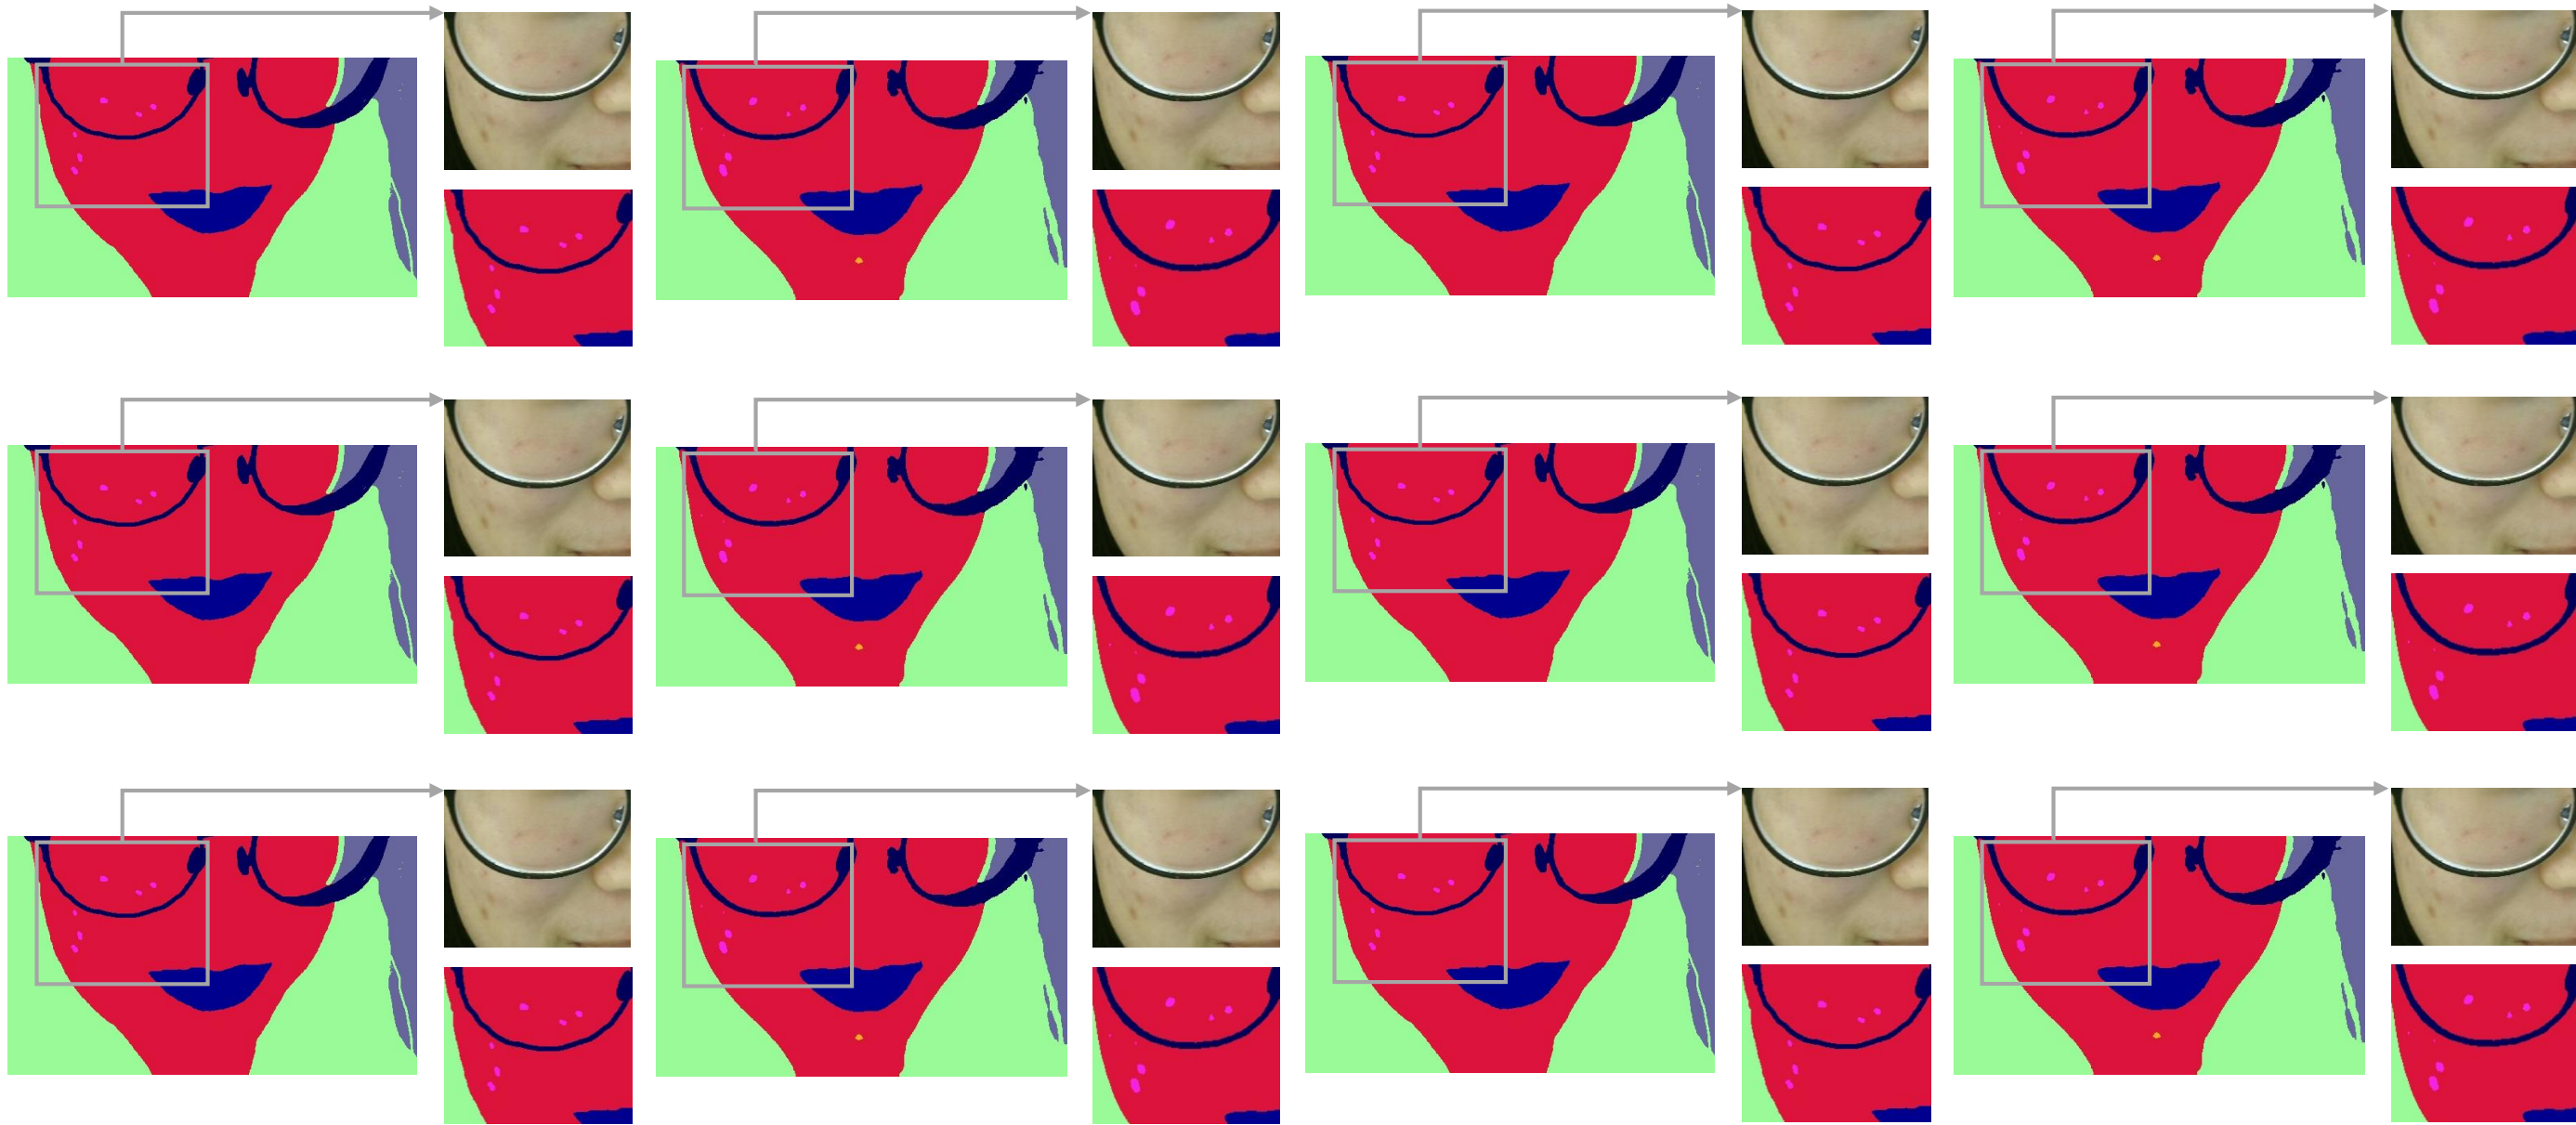



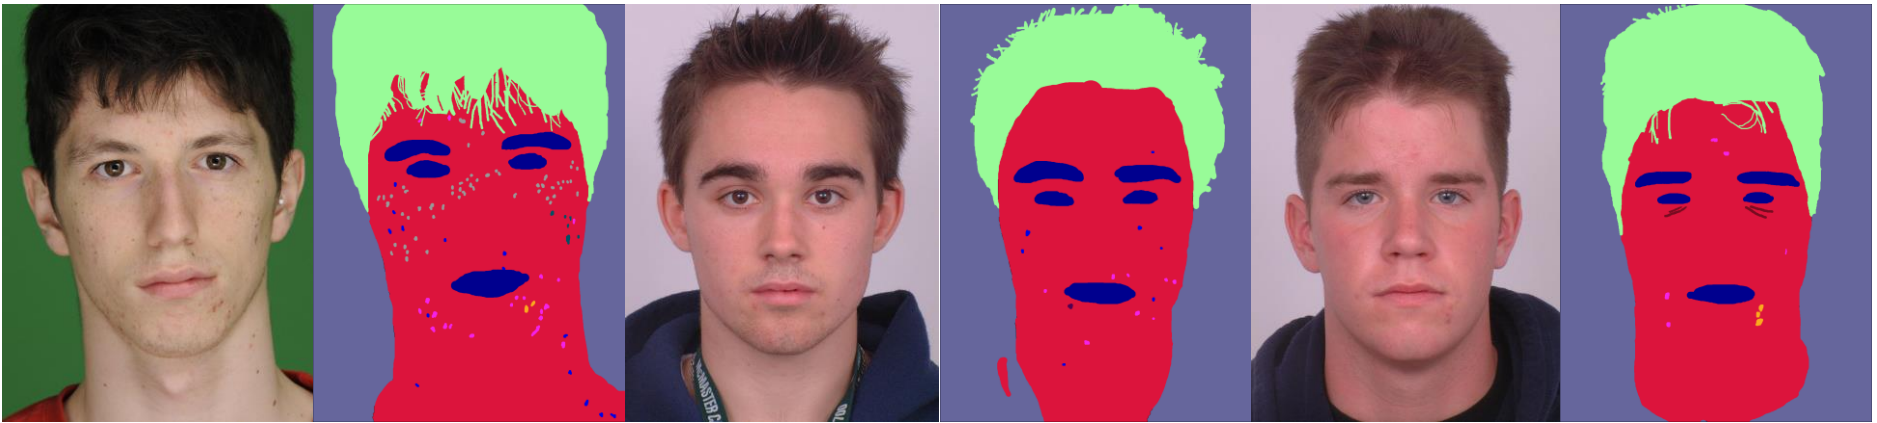

Image

Ground Truth

Image

Ground Truth

Image

Ground Truth

|         |           |          |         |                       |         |                     |             |            |
|---------|-----------|----------|---------|-----------------------|---------|---------------------|-------------|------------|
| papule  |           | age spot | PIH     | seborrheic dermatitis | dot     | scarf, mask         | hair        | glasses    |
| pustule | whitehead | freckle  | melasma | flush                 | wrinkle | mouth/eyes/eyebrows | normal skin | background |

acnes

pigments

redness

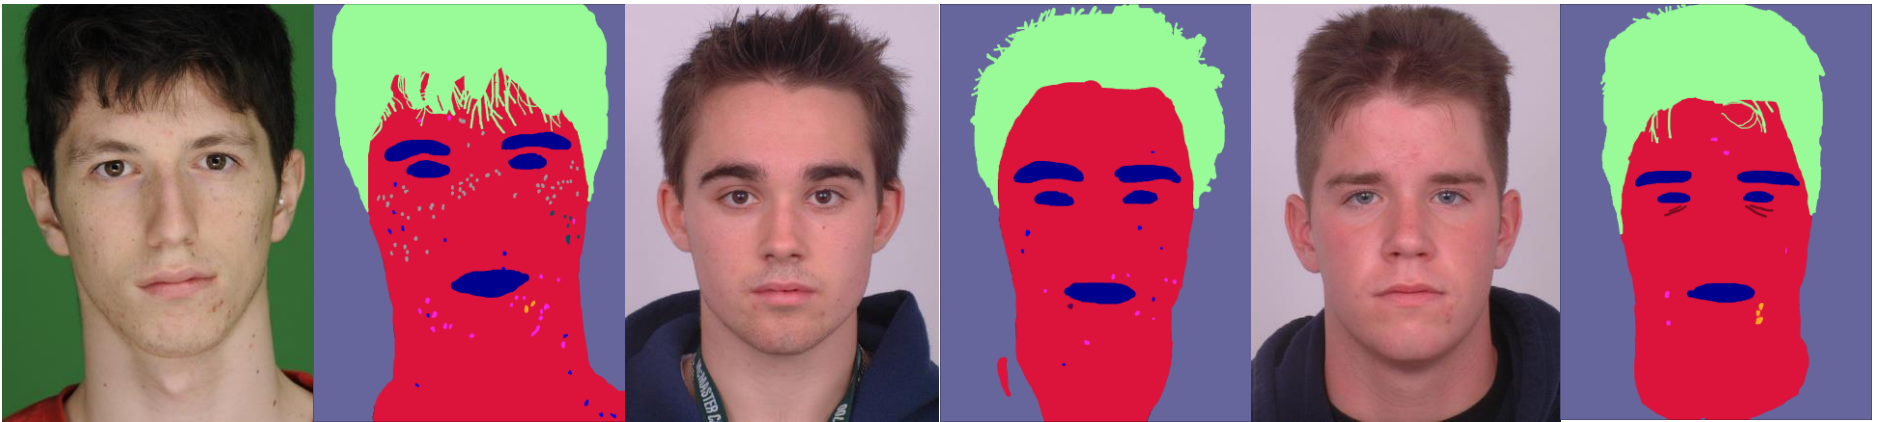

Image

Ground Truth

Image

Ground Truth

Image

Ground Truth

|        |           |          |         |             |             |                       |            |     |
|--------|-----------|----------|---------|-------------|-------------|-----------------------|------------|-----|
| papule | whitehead | age spot | pustule | freckle     | melasma     | seborrheic dermatitis | flush      | PIH |
| dot    | freckle   | hair     | glasses | normal skin | scarf, mask | mouth/eyes/eyebrows   | background |     |
